# Supplementary material for: Defects, parcellation, and renormalized negative diffusivities in non-homogeneous oscillatory media
Source: arXiv:2502.09264 source file (2025-09-19)
Supplement: Supplementary file 1 [file SupplementaryMaterial.pdf]

**Supplementary Material of**  
**“Defects, parcellation and renormalized negative diffusivities in non-homogeneous**  
**oscillatory media”**  
**by Marie Sellier-Prono, Massimo Cencini, David Kleinfeld, Massimo Vergassola**

**CONTENTS**

|      |                                                                                        |    |
|------|----------------------------------------------------------------------------------------|----|
| I.   | Comparison between peristalsis experimental data and our Ginzburg-Landau modeling data | 1  |
| II.  | Counting the number of frequency plateaus                                              | 3  |
| III. | Phase-space diagrams for the number of plateaus                                        | 5  |
| IV.  | The WKB method to quantify the profile of amplitude modulation                         | 6  |
| V.   | Discrete <i>vs</i> continuous models of coupled oscillators                            | 8  |
| VI.  | Re-derivations of results in Ref. [1] (Ref. [30] in the main paper)                    | 9  |
| A.   | Open boundaries                                                                        | 10 |
| 1.   | The resolvent                                                                          | 10 |
| 2.   | Asymptotic expansions of the Airy function $Ai$ for large arguments                    | 12 |
| B.   | One reflecting boundary                                                                | 13 |
| 1.   | The Wronskian                                                                          | 13 |
| 2.   | Poles of the resolvent and stability                                                   | 14 |
|      | References                                                                             | 15 |

**I. COMPARISON BETWEEN PERISTALSIS EXPERIMENTAL DATA AND OUR  
GINZBURG-LANDAU MODELING DATA**

*a. Experimental and numerical data.* Experimental data for Fig. 1 in the main text was extracted from [2] by using the WebPlotDigitizer software [3]. Specifically, the frequency data of Figs. 1a and 1c were taken from Fig. 5, and the time courses of Fig. 1b from Fig. 9 of [2]. Note that Figs. 5 and 9 of [2] refer to different experiments. Indeed, the paper does not provide time courses measured for the same experiment as in Fig. 5. Figures showing both time series and frequency measurements either lack the natural frequencies (measured in isolated chunks of the intestine) or provide time courses that are of insufficient image quality (erased lines) for data extraction. The reason we chose Fig. 9 is that it shows data qualitatively similar to other time courses represented in the paper, and it is the time series of the highest quality for extraction using [3]. Thus, we can demonstrate that both experimental frequency plateaus and time courses are similar to theoretical ones.

Numerical data is generated by integrating the following one-dimensional Ginzburg-Landau equation with a gradient in natural frequencies and an advective term

$$\partial_t A(x, t) + V \nabla A = r A (1 - |A|^2) + i(gx + \omega_0) A + D \Delta A, \quad (1)$$

with Neumann boundary conditions  $\nabla A(\pm L/2) = 0$ . The advective term does not appear in standard formulations of the GL equation where isotropy and parity hold. However, the presence of a gradient of frequencies makes it acceptable. Indeed, in one dimension, the gradient breaks parity, and therefore a term  $\propto \nabla A$  is possible. Note that the term respects the gauge invariance  $A \mapsto A e^{i\phi}$ . More generally, in the multi-dimensional case, a gradient of frequencies  $\mathbf{g}$  identifies a preferential direction that breaks isotropy, and a term  $\propto \mathbf{g} \cdot \nabla A$  is then acceptable.

We integrated Eq. (1) by time-marching it with Euler method and using a finite-difference scheme with fourth-order discretization of first and second spatial derivatives. Note that the advective term breaks the  $A(x) = \bar{A}(-x)$  symmetry of the equation without advection that was mostly discussed in the main text. Consequently, we must integrate over the whole domain  $[-L/2, L/2]$ . We use  $N = 1511$  collocation points, and the ratio of the time step  $\Delta t$  to the smallest

natural period satisfies  $\left| \frac{gL}{2\pi} \right| \Delta t < 10^{-2}$ . Simulations are performed for multiple values of  $\alpha \equiv L^3|g|/D$ ,  $\beta \equiv Dg^2/r^3$ ,  $Pe \equiv |V|L/D$ . Specifically, we investigated  $\alpha \in \{2 \times 10^{0.1(n-3)}, n \in \llbracket 0, 49 \rrbracket\}$ ,  $\beta \in \{10^n, n \in \llbracket -9, 3 \rrbracket\}$ ,  $Pe = 10$ ;  $\alpha \in \{2 \times 10^{0.1(n-3)}, n \in \llbracket 25, 49 \rrbracket\}$ ,  $\beta \in \{10^{n/2}, n \in \llbracket -3, 1 \rrbracket\} \cup \{0.01n, n \in \llbracket 4, 9 \rrbracket\}$ ,  $Pe \in \{10, 20\}$ . The frequency shift  $\omega_0$  is first set to zero.

*b. Comparison procedure.* The comparison between numerical and experimental data exploits that simulations with identical parameters  $\alpha$ ,  $\beta$ , and  $Pe$  are equivalent, up to rescalings in time and space and a shift in frequencies. We first compare natural and average frequency profiles obtained by numerics to those extracted from Fig. 5 of Ref. [2]. To identify potential candidates, we focused on the profiles' shapes (constant for given  $\alpha$ ,  $\beta$ , and  $Pe$ ) rather than trying to match frequency or length (which can be reproduced with suitable rescalings as detailed below). The matching procedure of a simulation of parameters  $g, D, L, r, V$  and  $\omega_0$  gives, through rescalings, the parameters  $g', D', L', r', V'$  and  $\omega'_0$  ( $\alpha = \alpha'$ ,  $\beta = \beta'$ ,  $Pe = Pe'$ ) that should be used in Eq. (1) to best capture the experimental data.

We chose to compare frequency profiles by imposing the superposition of natural frequency lines and trying to find the best possible match of average frequencies. Thus,  $g' = g_{exp}$  where  $g_{exp}$  is the experimental natural frequency gradient, which is extracted from Fig. 5 of Ref. [2]. Practically, the procedure consists of the following steps:

1. Find a good potential match of the experimental plateaus in Fig. 5 of Ref. [2] for a region of the numerical simulation domain.
2. **Space rescaling:** Put numerical and experimental data in the same reference frame, so that experimental data and the matching region of the simulation have the same coordinates. To do so, chose the coordinates  $x'_0, x'_1$  for the boundaries ( $x = \pm L/2$  in the original reference frame) of the numerical data in the reference frame of the experiment. The new simulation length is  $L' = x'_1 - x'_0$  and space is rescaled by  $x' = xL'/L$ .
3. **Time rescaling:** Matching the gradient of natural frequencies then imposes the rescaling of the simulation time:  $t' = t \frac{gL}{g'L'}$ .
4. **Frequency shift:** Finally, matching the natural frequencies imposes the frequency shift:  $\omega'_0 = \omega_{exp}(x' = 0) - \omega(x' = 0) \frac{g'L'}{gL}$ , where  $\omega_{exp}$  and  $\omega(x) = gx$  are the experimental and numerical natural frequencies.

Note that the change  $x \rightarrow -x$  in Eq. (1) amounts to changing the signs of  $g$  and  $V$ . All our simulations were performed with  $g > 0$  and  $V < 0$ , but the experimental gradient is negative, so we changed  $x'$  to  $-x'$  to perform the match. Thus, to obtain the best comparison parameters, negative  $g$  and positive  $V$  should be used, as shown in the rescaled and mirrored parameters of Table I. The parameters needed to obtain directly the rescaled simulation are given in Table I. However, integrating (1) with the rescaled parameters is too long. Therefore, to reduce computing time, we run simulations using original parameters and a frequency shift  $\omega'_0 \frac{gL}{g'L'}$  to match experimental frequencies, as results for both sets of parameters are equivalent up to space and time rescalings. Numerical data of Figs. 1a and 1c of the main text has been generated using parameters of Table I.

|                       | Non-dimensional parameters |                  |            | Simulations parameters |                    |                                         |                              |                         |                             |
|-----------------------|----------------------------|------------------|------------|------------------------|--------------------|-----------------------------------------|------------------------------|-------------------------|-----------------------------|
| Original              | $\alpha$                   | $\beta$          | $Pe$       | $g$ (rad/s)            | $L$ (m)            | $r$ (s <sup>-1</sup> )                  | $D$ (m <sup>2</sup> /s)      | $V$ (m/s)               | $\omega_0$ (rad/s)          |
|                       | 1000                       | 0.07             | 10         | 501.2                  | 1                  | 121.5                                   | 0.5                          | -5                      | 0                           |
| Rescaled and mirrored | $\alpha' = \alpha$         | $\beta' = \beta$ | $Pe' = Pe$ | $g' = g_{exp}$         | $L' = x'_1 - x'_0$ | $r' = \frac{g'L'}{(\alpha\beta)^{1/3}}$ | $D' = \frac{g'L'^3}{\alpha}$ | $V' = Pe \frac{D'}{L'}$ | $\omega'_0$                 |
|                       | 1000                       | 0.07             | 10         | -1.25                  | 0.479              | 0.1452                                  | $1.371 \times 10^{-4}$       | $2.286 \times 10^{-3}$  | 1.452                       |
| Used                  | $\alpha$                   | $\beta$          | $Pe$       | $g$                    | $L$                | $r$                                     | $D$                          | $V$                     | $\omega'_0 \frac{gL}{g'L'}$ |
|                       | 1000                       | 0.07             | 10         | 501.2                  | 1                  | 121.5                                   | 0.5                          | -5                      | 1200.14                     |

TABLE I. Parameters used in simulations to match experimental data of Fig.5 of [2] and values for the best match shown in Fig. 1 of the main text. Original: parameters used in the exploration phase, looking for potential matches. Rescaled and mirrored: parameters to best reproduce experimental data, computed using the matching procedure and changing the signs of  $g$  and  $V$ , which amounts to mirroring the simulation ( $x' \rightarrow -x'$ ). Used: parameters used in the simulation shown in Fig. 1 of the main text, equivalent up to time and space rescalings to the rescaled and unmirrored parameters.

## II. COUNTING THE NUMBER OF FREQUENCY PLATEAUS

In Fig. 2 of the main text, we showed that the number of frequency plateaus,  $N_p$ , scales linearly with  $\alpha^{1/3}$ , for different values of  $\beta$ . In this Section, we detail the methods used to estimate  $N_p$ . Referring to Figs. 2b and 2c in the main text, we can already observe some challenges: while the plateaus may be clearly defined (“clean” as in Fig. 2c), they can also be poorly defined (“unclean” as in Fig. 2b). It is not immediately obvious how to count the latter. This issue is further illustrated in Fig. 1, which shows examples of plateaus for various values of  $\alpha$  and  $\beta$  with both Dirichlet (upper panels) and Neumann (lower panels) boundary conditions.

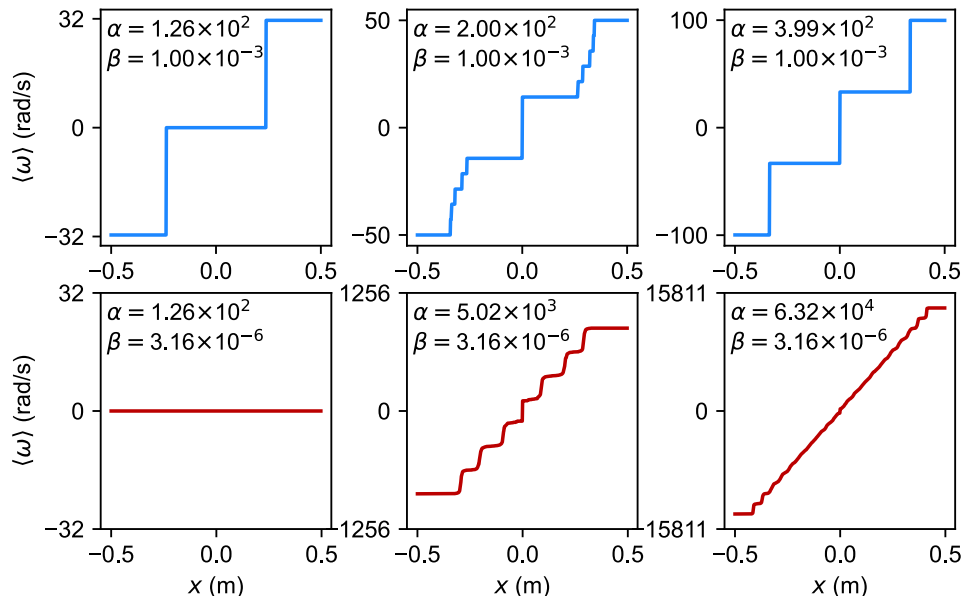

FIG. 1. Examples of average frequency plateaus obtained for both types of boundary conditions. Note that clean and unclean plateaus are observed with both boundary conditions. Top (blue): Dirichlet boundary conditions. In the transition from  $N_p = 3$  (left) to  $N_p = 4$  (right), smaller transitional plateaus appear between large ones (middle). Bottom (red): Neumann boundary conditions. The minimal number of plateaus is 1 (full locking, left), increasing indefinitely with  $\alpha$ . Some plateaus are not “clean”, complicating their counting (middle and right).

The presence of clean and unclean plateaus was observed previously in Refs. [4, 5] for a discrete analog of the Ginzburg-Landau equation, and in Refs. [6, 7]. In particular, Ref. [6] investigated numerically plateaus and observed that regions of clean plateaus shrink as  $L$  increases, and are surrounded by regions where plateaus are unclean. Ref. [7] suggested that unclean plateaus are associated with chaotic motion.

In our simulations, we did not specifically investigate the chaotic nature of unclean plateaus, as this issue lies outside the primary scope of our work. However, we did observe that, for certain values of  $\alpha$  and  $\beta$ , defects – after an initial transient – tend to appear periodically at the same locations, leading to clean plateaus. For other values, defects seem to move, either periodically or irregularly, resulting in unclean plateaus. It is also worth noting that in all our simulations, which start with  $A(x, 0) = 1$  for all  $x$ , we disregarded the transient dynamics when calculating the average frequency. This is because, during the transient phase, defects can sometimes exceed their asymptotic number, or have some transient irregularities.

As discussed earlier, counting clean plateaus is straightforward, but becomes less clear in other cases. To address this issue, we tested the following two different procedures.

**Method 1** relies on the observation (see also Ref. [5]) that usually (in particular for Dirichlet boundary conditions), clean plateaus have equal frequency jumps  $\delta\omega = gL/N_d$  between adjacent plateaus. Here,  $N_d$  is the number of defects related to the number of plateaus as  $N_p = N_d + 1$ . The idea is then to estimate  $\delta\omega$  from the plot of  $\langle \omega(x) \rangle$ . Although this method can be challenging and occasionally ambiguous, it is effective in the case of Dirichlet boundary conditions. This is because plateaus near the left boundary are always well-defined, with an average frequency  $-gL/2$ , as imposed by the left boundary condition. Therefore, one only needs to identify the region corresponding to adjacent plateaus and fit the average frequency within that region.

**Method 2** uses the clustering algorithm OPTICS [8] to find clusters of synchronization. The input data is the correlation matrix,  $R$ , which measures how much two given points oscillate with a constant phase shift on average.

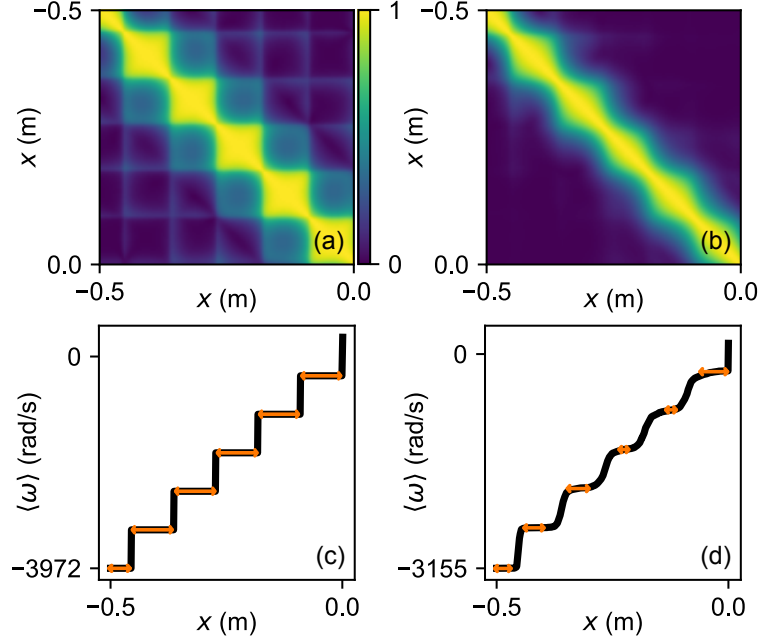

FIG. 2. The clustering algorithm for plateaus' identification. (a) and (b): Matrix  $R$  of phase correlations in the left half of the simulation domain (the right half is symmetric). (c) and (d): Average frequency (black line) and clusters found by the OPTICS algorithm (arrows) in the left half of the system. Both panels are using Dirichlet boundary conditions, with  $\alpha = 1.589 \times 10^4$  and  $\beta = 3.16 \times 10^{-3}$  for (a) and (c);  $\alpha = 1.262 \times 10^4$  and  $\beta = 3.16 \times 10^{-4}$  for (b) and (d).

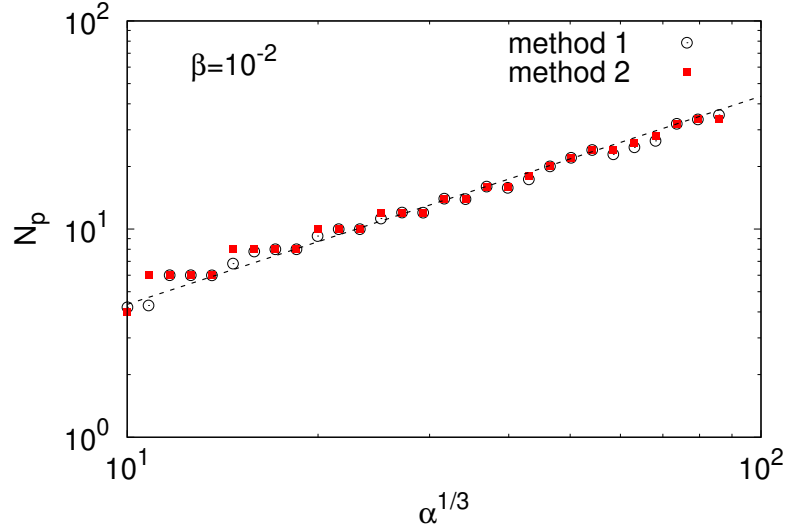

FIG. 3. Robustness of the 1/3 scaling of the number of plateaus. Number of plateaus,  $N_p$ , vs  $\alpha^{1/3}$  for  $\beta = 10^{-2}$  and Dirichlet boundary conditions, computed using the two methods described in the text. The dashed line highlights the power-law dependence  $N_p \propto \alpha^{1/3}$  predicted in the main text.

Its elements are computed as

$$R_{jk} = \frac{1}{T} \sum_{t=0}^T \left| e^{i(\phi_j(t) - \phi_k(t))} \right|, \quad (2)$$

where  $T$  is the duration of the simulation interval (with transients removed), and  $\phi_k(t)$  is the phase of the oscillator at position  $x = k\Delta x$  and time  $t$ . The matrix  $R$ , shown in Figs. 2a,b, is then given as input to the OPTICS algorithm,

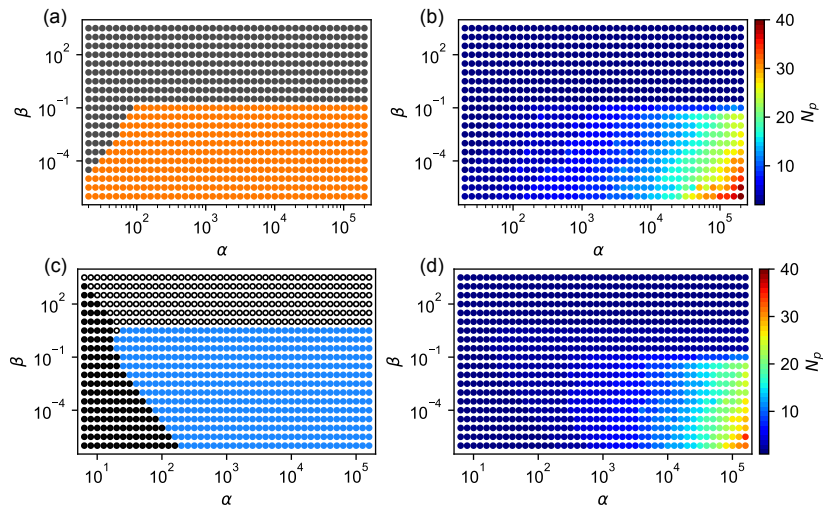

FIG. 4. Variation of the number of plateaus  $N_p$  in the  $(\alpha, \beta)$  phase space.  $N_p$  is measured by using the OPTICS algorithm described previously. The panels (a) and (b) refer to Dirichlet boundary conditions, while (c) and (d) refer to Neumann ones. Colors in panels (a) and (c) discriminate between regions with the minimal number of plateaus allowed and the rest of the phase space. In (a), the minimal number is  $N_p = 2$  (gray) vs  $N_p > 2$  (orange), while in (c),  $N_p = 1$  (black) vs  $N_p > 1$  (blue). Empty circles in (c) denote the region of oscillator death where  $A = 0$  is stable and eventually attained. Panels (b) and (d) highlight the complementary information about the number of plateaus in the regions where several of them are present.

which identifies the plateaus (phase-coherent regions on average). The choice of OPTICS over other clustering algorithms was motivated by three main arguments. First, OPTICS is a density-based clustering algorithm that uses soft clustering: it finds clusters of points close in the space of pairwise coherence and will not classify outliers. In our case, outliers are points at which space-time defects usually appear. Second, it can find clusters of different densities in the same dataset. It allows us to find all clusters, even in those cases where some clusters have worse synchronization than others; for instance, the second cluster in Fig. 2d would be denser in the space of pairwise correlations than the fourth one. Third, hyperparameters do not include the number of clusters, which is sometimes difficult to determine by eye, so we can let the algorithm make an unbiased and objective estimation. This is particularly important as we are interested in the evolution of the number of clusters.

Like the first, Method 2 is straightforward and unambiguous for clean plateaus but becomes more moot for unclear plateaus. The key advantage of Method 2 is its objectivity, which is why we used it to present results in the main paper. Notably, for most parameter values, the two methods agree reasonably well and, most importantly, yield the same scaling behavior of  $N_p$  vs  $\alpha^{1/3}$ , as shown in Fig. 3 for Dirichlet boundary conditions for  $\beta = 10^{-2}$ .

### III. PHASE-SPACE DIAGRAMS FOR THE NUMBER OF PLATEAUS

As discussed in the main text, the number of plateaus and the corresponding defects vary substantially with the two non-dimensional parameters  $\alpha \equiv L^3|g|/D$  and  $\beta \equiv Dg^2/r^3$  defined by Eq. (4) in the main text. There, we concentrated on deriving the  $1/3$  scaling law for the number of plateaus  $N_p$  as a function of  $\alpha$  in the regime of small  $\beta$ 's. Here, Fig. 4 aims to provide a less quantitative but more global view of  $N_p$  variations in the phase space.

The lower-right corner of the phase space (large  $\alpha$  and small/moderate  $\beta$ ) is the region where  $N_p$  is large. Statistical arguments developed in the main text apply, together with the consequent  $1/3$  law for  $N_p$  vs  $\alpha$ . As already noted, the law applies to both boundary conditions, which is also visually confirmed by Fig. 4. As  $\beta$  increases,  $N_p$  first reduces to a handle of plateaus and eventually to the minimal number for the corresponding boundary conditions, as shown in Fig. 4. The boundary of the transition to the minimal number (or the oscillator death state for Neumann conditions) is highlighted in panels (a) and (c). Specifically, the upper-right corner is the region of oscillator death for Neumann boundary conditions and WKB asymptotics for Dirichlet boundary conditions. Note that oscillator death at moderately large  $\alpha$  is reached (see Fig. 4d) in a non-monotonic way as  $\beta$  increases: the locked region (black) first transitions to multiple plateaus (blue) and eventually to oscillator death (empty circle).

For Dirichlet boundary conditions, the main text concentrated on the derivation of WKB asymptotics for large  $\alpha$  and  $\beta$ . The next Section generalizes the analysis to the region visible in Fig. 4a of large  $\alpha$  and moderate  $\beta$ 's, where two plateaus are still present.

#### IV. THE WKB METHOD TO QUANTIFY THE PROFILE OF AMPLITUDE MODULATION

As in the main text, we consider the (real) GL equation

$$\partial_t A = (r + i\omega) A - r|A|^2 A + D\Delta A, \quad (3)$$

with a uniform gradient  $\omega(x) = gx$ , where we can add or subtract an average frequency without any loss of generality. The Dirichlet boundary conditions are  $A(\pm L/2, t) = e^{\pm igLt/2}$ , with the symmetry of the real and imaginary parts,  $\text{Re } A(-x) = \text{Re } A(x)$  and  $\text{Im } A(-x) = -\text{Im } A(x)$ , with respect to the origin.

We consider the region of the phase diagram in Fig. 4a where numerical evidence indicates that the system locks into two frequency clusters, at the frequencies  $-gL/2$  and  $+gL/2$  on the left and the right of the origin, respectively. A defect at the origin is generated periodically with period  $2\pi/gL$ , corresponding to the frequency difference between the two clusters. This is well visible in Movie 1, which shows the evolution of the amplitude and the phase for  $\alpha = 4 \times 10^4$  and  $\beta = 1$ . The phase gradient diverges at the origin, until the amplitude goes to zero and the phase jumps to reset the gradient. Note that a shift in frequencies of  $gL/2$  has been performed in the movie. This is because our following analysis focuses on the left region  $-L/2 \leq x \leq 0$  (the other side being obtained by the above symmetry). Adding to the frequencies  $gL/2$ , i.e., defining  $A \equiv \tilde{A}e^{-igtL/2}$ , the solution  $\tilde{A}$  takes a static form, except for a region around the origin, which shrinks as  $g$  increases (see Fig. 5).

Our goal here is to detail how the above static solution is obtained by using the WKB approximation. We focus on the region where  $|A| \ll 1$  so that we can neglect non-linear terms. Eq. (3) reduces then to

$$0 = \frac{1}{D} (r + ig\tilde{x}) \tilde{A} + \Delta \tilde{A}; \quad \tilde{x} \equiv x + \frac{L}{2}. \quad (4)$$

In the limit  $\beta = Dg^2/r^3 \gg 1$ , which we consider first, we can neglect the  $r$  term and the equation further reduces to

$$0 \simeq \left[ \frac{ig\tilde{x}}{D} + \Delta \right] \tilde{A}. \quad (5)$$

This is the case considered in the main text, which we detail here for completeness. We will then move on to moderate  $\beta$ 's.

The usual WKB procedure [9] is to pose  $\tilde{A} = e^\psi$ , which yields  $\Delta \tilde{A} = (\psi'^2 + \psi'') e^\psi$ , and then use the expansion  $\psi = \psi_0 + \psi_1 + \dots$  with the condition  $\psi'' \ll \psi'^2$  (to be verified *a posteriori*), to obtain

$$(\psi'_0)^2 \simeq -\frac{ig\tilde{x}}{D}; \quad \psi'_1 \simeq \left( -\frac{1}{2} \log \psi'_0 \right)'. \quad (6)$$

The solution to the first equation that decays as  $x$  increases is (apart from an irrelevant constant):

$$\psi_0 = \frac{2}{3} \sqrt{-i\frac{g}{D}} \tilde{x}^{3/2} = \begin{cases} \frac{2}{3} \sqrt{\frac{g}{D}} e^{i\frac{3\pi}{4}} \tilde{x}^{3/2} & \text{for } g > 0, \\ \frac{2}{3} \sqrt{\frac{|g|}{D}} e^{-i\frac{3\pi}{4}} \tilde{x}^{3/2} & \text{for } g < 0. \end{cases} \quad (7)$$

The solution to the second is

$$\psi_1 = -\frac{1}{4} \log \tilde{x}. \quad (8)$$

We conclude that the original function  $A$  decays like

$$A \simeq e^{-i\frac{gtL}{2}} \frac{e^{-\sqrt{\frac{2g}{9D}}(1-i\text{sgn}(g))(x+\frac{L}{2})^{3/2}}}{(x + \frac{L}{2})^{1/4}}, \quad (9)$$

which is the expression reported in the main text.

For the method to work consistently, it should be true that  $\psi'' \ll \psi'^2$ , which amounts to  $\sqrt{\frac{|g|}{D\tilde{x}}} \ll \frac{|g|}{D}\tilde{x}$ , i.e., that the argument at the exponential is large:  $\tilde{x} \gtrsim (D/|g|)^{1/3}$ . Since the entire domain has extension  $L$ , a necessary condition for the validity of the asymptotics is that the pure number  $\alpha = |g|L^3/D \gg 1$ . The other approximation

of neglecting  $r$  with respect to  $gx$  in the region of asymptotics entails  $r \ll |g|(D/|g|)^{1/3}$ , i.e., the non-dimensional number  $\beta = Dg^2/r^3 \gg 1$ .

The approximation eventually breaks down as  $x$  approaches the origin because time-dependent effects in the original equation become important (see the attached Movie 1). These are due to the fact that the boundary condition at the origin is dictated by the requirement of symmetry and should accommodate the other side of the domain that varies with a different time-dependence. That is the origin of the periodic shedding of defects. For large  $|g|$ , the applicability of Eq. (9) becomes wider and wider, as shown in Fig. 5.

If the non-dimensional number  $\beta = Dg^2/r^3$  is not large, then WKB still applies, yet the linear  $rA$  term ought to be kept, which leads to the following (more involved) calculations. We pose again  $A = e^{-igLt/2}e^\psi$ , which yields  $\Delta A = (\psi'^2 + \psi'')e^\psi$ . One then uses the perturbative expansion  $\psi = \psi_0 + \psi_1 + \dots$  with the usual WKB approximation  $\psi'' \ll \psi'^2$ , to obtain that Eqs. (6) are modified as

$$(\psi'_0)^2 \simeq -\frac{r + ig\tilde{x}}{D}; \quad \psi'_1 \simeq \left(-\frac{1}{2} \log \psi'_0\right)'. \quad (10)$$

The second equation is immediately solved as

$$\psi_1 = -\frac{1}{2} \log(\psi'_0) + \text{const.} \quad (11)$$

As for the first one, we have (we remind that  $r$  is taken real)

$$\psi'_0 = \frac{1}{\sqrt{D}} (r^2 + g^2\tilde{x}^2)^{1/4} e^{i(\frac{\pi}{2} + \frac{\chi}{2})\text{sgn}(g)}, \quad (12)$$

where  $\cos \chi = r/\sqrt{r^2 + g^2\tilde{x}^2}$  and  $\sin \chi = |g|\tilde{x}/\sqrt{r^2 + g^2\tilde{x}^2}$ . Here, we have shifted the original angle (in the third quadrant for  $g > 0$  and the second for  $g < 0$ ) to the first quadrant (whence the  $i\pi/2$  at the exponential) so that the square root leaves the half-angle in the same respective domains. It follows that

$$\cos\left(\frac{\chi}{2}\right) = \sqrt{\frac{1 + \cos \chi}{2}} = \frac{\sqrt{\sqrt{r^2 + g^2\tilde{x}^2} + r}}{\sqrt{2}(r^2 + g^2\tilde{x}^2)^{1/4}}; \quad \sin\left(\frac{\chi}{2}\right) = \sqrt{\frac{1 - \cos \chi}{2}} = \pm \frac{\sqrt{\sqrt{r^2 + g^2\tilde{x}^2} - r}}{\sqrt{2}(r^2 + g^2\tilde{x}^2)^{1/4}}. \quad (13)$$

Note that the other possible determination of the square root would have  $i\pi/2$  at the exponential in Eq. (12) changed into  $3i\pi/2$ , which would lead to a non-acceptable monotonously increasing real part.

Collecting the various terms, we have

$$\begin{aligned} \psi_0 &= -\frac{1}{\sqrt{2D}} \left[ \int^{\tilde{x}} \sqrt{\sqrt{r^2 + g^2y^2} - r} dy \mp i \int^{\tilde{x}} \sqrt{\sqrt{r^2 + g^2y^2} + r} dy \right] \\ &= -\frac{r^{3/2}}{|g|\sqrt{2D}} \left[ \int^{|g|\tilde{x}/r} \sqrt{\sqrt{1 + u^2} - 1} du \mp i \int^{|g|\tilde{x}/r} \sqrt{\sqrt{1 + u^2} + 1} du \right]. \end{aligned} \quad (14)$$

The upper/lower sign of the imaginary part applies to  $g$  positive/negative, respectively. The change of variable  $\sqrt{1 + u^2} \equiv z$  reduces the two above integrals to known forms

$$\int^x \frac{z}{\sqrt{z+1}} dz = \frac{2}{3} (x-2) \sqrt{1+x}; \quad \int^x \frac{z}{\sqrt{z-1}} dz = \frac{2}{3} (x+2) \sqrt{x-1}. \quad (15)$$

These expressions are obtained by adding and subtracting one at the numerator, which reduces both integrals to the sum of two elementary fractional powers.

By using (15) into (14) modified by the change of variable to  $z$ , we finally obtain

$$\begin{aligned} \psi_0 &= -\sqrt{\frac{2r^3}{9Dg^2}} \left\{ \left[ \left( \sqrt{1 + \left(\frac{g\tilde{x}}{r}\right)^2} - 2 \right) \sqrt{\sqrt{1 + \left(\frac{g\tilde{x}}{r}\right)^2} + 1} \right] \right. \\ &\quad \left. \mp i \left[ \left( \sqrt{1 + \left(\frac{g\tilde{x}}{r}\right)^2} + 2 \right) \sqrt{\sqrt{1 + \left(\frac{g\tilde{x}}{r}\right)^2} - 1} \right] \right\}. \end{aligned} \quad (16)$$

In the limit  $g\tilde{x}/r \gg 1$ , it is checked that we recover the previous results, Eqs. (7) and (9).

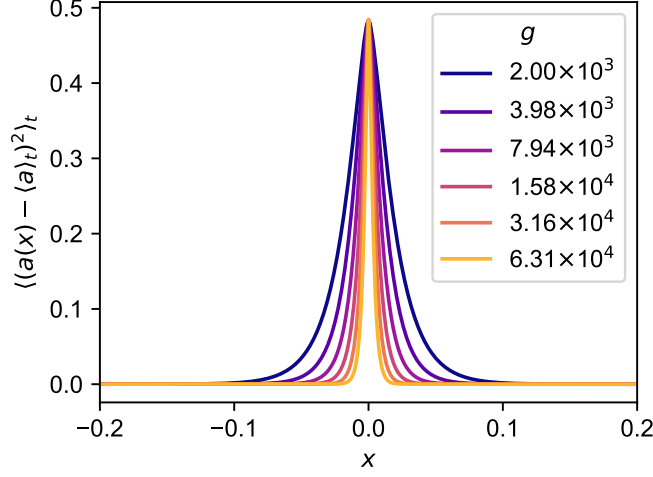

FIG. 5. Enlargement of the region of applicability of the WKB asymptotics as  $|g|$  increases. We quantified non-stationary effects by the standard deviation of the amplitude over a cycle of the defects' appearance at the origin. The standard deviation of the amplitude  $a$  of the field  $A$  is almost vanishing over most of the domain  $[-1/2, 1/2]$  (not entirely shown for easier visualization). That reflects the quasi-stationarity of the two regions locked at  $\mp gL/2$  at the left/right of the origin. Amplitude variations in time are restricted to a region around the origin (where defects periodically appear), which is zoomed in for the figure. Simulations were obtained for Dirichlet boundary conditions, and parameters  $D = 0.5$ ,  $L = 1$ ,  $\beta = 1$  and  $r$  is obtained for each value of  $g$  in the plot as  $r = (Dg^2/\beta)^{1/3}$ .

## V. DISCRETE VS CONTINUOUS MODELS OF COUPLED OSCILLATORS

The existence of frequency plateaus in oscillator chains has been known for a long time and was mostly investigated in the framework of weakly-coupled oscillators [10]. These studies mainly focused on phase oscillators, i.e., they neglected the amplitude. As discussed in the main text, zeros of the amplitude, i.e., defects, are an important feature of frequency plateaus in the inhomogeneous Ginzburg-Landau equation. Defects are, of course, absent in phase oscillators. This Section discusses the relationship between the two approaches and conditions under which the approximation of weakly-coupled oscillators can still be justified.

We consider the space-discretized form Eq. (1) of the main text

$$\partial_t A_k = i g (Lk/N) A_k + r A_k (1 - |A_k|^2) + (DN^2/L^2)(A_{k+1} - 2A_k + A_{k-1}), \quad (17)$$

with  $k = -N/2, \dots, N/2$ , and no-flux boundary conditions, i.e.  $A_{-N/2} = A_{-N/2+1}$  and  $A_{N/2} = A_{N/2-1}$ . As in the main text, we can write  $A_k = a_k e^{i\phi_k}$  and obtain the discretized amplitude and phase equations:

$$\dot{a}_k = r a_k (1 - a_k^2) + \frac{DN^2}{L^2} (a_{k+1} \cos(\phi_{k+1} - \phi_k) - 2a_k + a_{k-1} \cos(\phi_k - \phi_{k-1})), \quad (18)$$

$$\dot{\phi}_k a_k = gL \frac{k}{N} a_k + \frac{DN^2}{L^2} (a_{k+1} \sin(\phi_{k+1} - \phi_k) - a_{k-1} \sin(\phi_k - \phi_{k-1})), \quad (19)$$

which are the discrete versions of Eqs. (2) and (3) in the main text.

It follows from the discretized equations above that the limit of weakly-coupled oscillators is violated in the continuum limit ( $N \rightarrow \infty$ ), as already noted in [11]. The suppression of amplitude modulation would require scaling the diffusion coefficient as  $D \sim 1/N^2$ , which seems difficult to motivate. We may still wonder whether the two descriptions can be matched in some appropriate limit, which is our goal hereafter.

Fig. 3 of the main text shows that a nonlinear locking region is present in the limit  $\beta = Dg^2/r^3 \rightarrow 0$ , i.e., for strong nonlinearity. In this limit, the amplitude of the oscillators is close to unity. Enforcing the approximation  $a_k \simeq 1$  in Eq. (18-19) reduces the equation for the phase to:

$$\dot{\phi}_k = gL \frac{k}{N} + \epsilon (\sin(\phi_{k+1} - \phi_k) - \sin(\phi_k - \phi_{k-1})), \quad (20)$$

where  $\epsilon = DN^2/L$ , and  $\phi_{-N/2} = \phi_{-N/2+1}$  and  $\phi_{N/2} = \phi_{N/2-1}$ . Eq. (20) was studied in Ref. [12] with  $gL = 1$ , while varying both  $N$  and  $\epsilon$ . With  $N$  fixed,  $\epsilon$  was increased from 0 to a critical value  $\epsilon_c(N)$  that scales linearly



with  $N$  (see also [11]). It was shown that there is a transition from a regime where all oscillators oscillate at their natural frequency to a frequency-locked regime, in which the number of plateaus (synchronized clusters) decreases as  $\epsilon$  increases. Then, at  $\epsilon \geq \epsilon_c(N)$ , a phase-locked regime is reached, where the entire chain of oscillators is synchronized. Since  $\epsilon_c \sim N$ , we conclude that only the phase-locked regime exists in the continuum limit  $N \rightarrow \infty$ . In the left panel

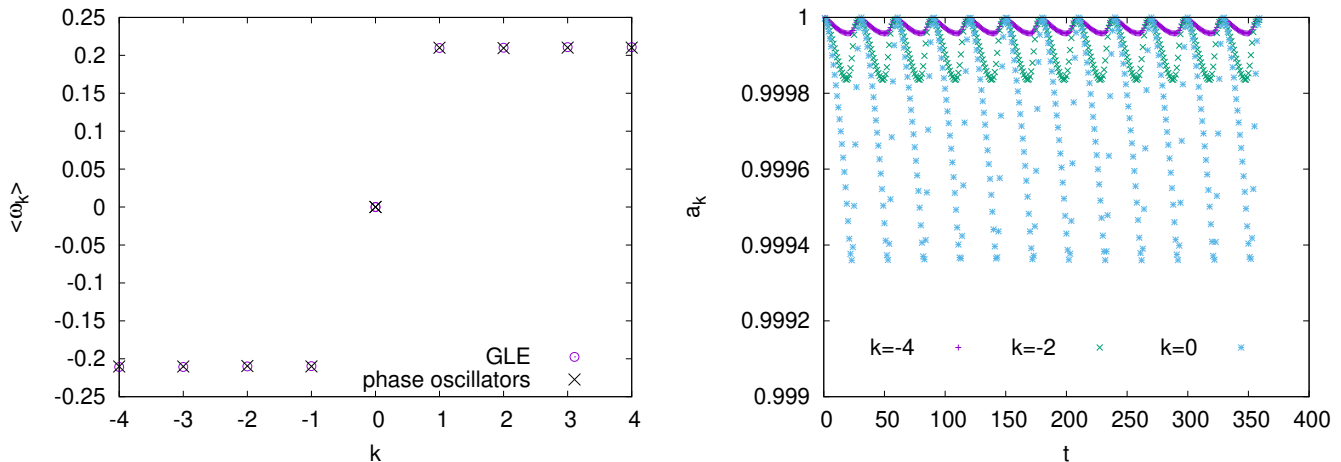

FIG. 6. Frequency plateaus in the discrete model Eq. (17): (left) The average frequency  $\langle \omega_k \rangle = \lim_{t \rightarrow \infty} \phi_k/t$  vs  $k$  for  $k \in [-N/2 : N/2]$  with  $N = 8$  for Eq. (17) with  $D = 0.005$ ,  $r = 10^3$ ,  $g = L = 1$  and for Eq. (20) with  $g = L = 1$  and  $\epsilon = DN^2/L = 0.32$ . (right) The time evolution of the amplitudes  $a_k$  of Eq. (19) for  $k = -4, -2, 0$  ( $k = 2, 4$  are equal by symmetry), showing that the approximation  $a_k \approx 1$  is well satisfied.

of Fig. 6, we show the average frequency of oscillations for  $N = 8$  obtained by simulating Eqs. (20) and (17), that is,  $N$  coupled Stuart-Landau oscillators. The frequency plateaus obtained with the two descriptions coincide and, as shown in the right panel, the amplitudes of the oscillators are close to unity (with  $O(1/r)$  corrections that are captured by perturbation analysis in the  $r \rightarrow \infty$  limit), and defects are not visible. In the continuum limit  $N \rightarrow \infty$ , both systems reach the phase-locked regime. Therefore, we can also interpret the phase-locked regime as the large coupling limit of the discrete (phase oscillator) model.

## VI. RE-DERIVATIONS OF RESULTS IN REF. [1] (REF. [30] IN THE MAIN PAPER)

The goal of this Section is to re-derive results obtained in [1], namely the dash-dotted line that appears in Fig. 3C of the main body of the paper, which corresponds to the result for a semi-infinite domain (see Eqs. (60)-(61) below).

Ref. [1] considers (Eq. (2.2) in the paper) the Bloch-Torrey [13, 14] equation with a unit gradient of frequencies:

$$\frac{\partial S(x, t)}{\partial t} = \frac{\partial^2 S(x, t)}{\partial x^2} + ixS(x, t). \quad (21)$$

A brief discussion of its importance for nuclear magnetic resonance and its physical meaning is presented in the body of the paper and will not be repeated here. Comparison with Eq. (7) in the body of our paper shows: 1) There is a change in notation with  $A$  in Eq. (7) being replaced by  $S$  here; 2) The growth term  $r'$  is absent. To cope with these differences we shall: 1) Keep using the notation  $S$  throughout this Section to conform with Ref. [1] and facilitate comparison with it; 2) Indicate along the way how to modify original derivations for our case Eq. (7) with  $r' \neq 0$ . For future reference, we rewrite it here as

$$\frac{\partial S(x, t)}{\partial t} = \frac{\partial^2 S(x, t)}{\partial x^2} + (r' + ix)S(x, t), \quad (22)$$

with the non-dimensional parameter  $\alpha$  defined in Eq. (4) of our main text set to unity to match Eq. (21). Note that the symbol  $\alpha$  is used in Ref. [1] to denote  $\alpha \equiv 2\pi/3$ . To avoid confusion, we shall therefore conform to this notation and, for this Section only, not refer any longer to the non-dimensional parameter  $\alpha$  defined by Eq. (4) of our main text.

### A. Open boundaries

Eq. (21) for its Laplace transform  $\hat{S}(x, s) \equiv \int_0^\infty e^{-st} S(x, t) dt$  reads :

$$(s - ix) \hat{S} - \frac{\partial^2 \hat{S}}{\partial x^2} = S(x, 0), \quad (23)$$

where the right-hand side arises from the boundary term of the integration by parts of the term  $\int_0^\infty \left(\frac{\partial S}{\partial t}\right) e^{-st} dt$ . Note that, at this stage, we are not taking into account any spatial boundary, which will be the subject of later Sections.

#### 1. The resolvent

A standard method to solve linear equations, such as Eq. (23), is to introduce the resolvent  $\hat{G}(x, y; s)$ , which solves

$$\left(s - ix - \frac{\partial^2}{\partial x^2}\right) \hat{G} = \delta(x - y). \quad (24)$$

To solve Eq. (24), we use that multiplication by  $x$  amounts to a derivative in Fourier space. We therefore introduce the Fourier transform

$$\hat{G}(x, y; s) \equiv \frac{1}{2\pi} \int e^{iqx} \hat{H}(q, y; s) dq, \quad (25)$$

and note that the equation for  $\hat{H}$  is

$$\left(s + \frac{\partial}{\partial q} + q^2\right) \hat{H} = e^{-iqy}. \quad (26)$$

The solution of this non-homogeneous equation is obtained by variation of constants as

$$\hat{H} = e^{-sq - q^3/3} \int^q e^{-iky} e^{sk + k^3/3} dk. \quad (27)$$

The expression of the original resolvent is then

$$\hat{G}(x, y; s) = \frac{1}{2\pi} \int_{-\infty}^{+\infty} e^{iqx} e^{-sq - q^3/3} dq \int_{-\infty}^q e^{-iky} e^{sk + k^3/3} dk = \frac{1}{2\pi} \int_{-\infty}^{+\infty} e^{-iqy} e^{sq + q^3/3} dq \int_q^\infty e^{ikx} e^{-sk - k^3/3} dk, \quad (28)$$

where for the last step we have exchanged the order of integration and then renamed the two variables of integration  $q \leftrightarrow k$ . The final expression coincides with (2.12) in Ref. [1]. Since the integrand is analytical, the integral over  $q$  that runs along the real axis can be deformed along big semi-circles either in the upper or the lower half-plane ( $C_1$  and  $C_{-1}$  in Ref. [1]). If  $q$  is moved to the complex plane, then the path from  $q$  to  $\infty$  starts from  $q$  and extends to infinity along the real axis (or, deforming again the path by analyticity, extends to infinity in the first sextant  $(-\pi/6, +\pi/6)$  where  $\exp(-k^3/3) \rightarrow 0$  as  $|k| \rightarrow \infty$ ).

In the case of our equation (7) in the body of the paper, the procedure for Eq. (22) is the same as above and the formula for the resolvent is simply modified as

$$\hat{G}(x, y; s) = \frac{1}{2\pi} \int_{-\infty}^{+\infty} e^{-iqy} e^{(s-r')q + q^3/3} dq \int_q^\infty e^{ikx} e^{-(s-r')k - k^3/3} dk, \quad (29)$$

with the same comments on the contours made above.

The behavior along the semicircles is captured by asymptotic analysis, namely by using the method of steepest descent. Its basic idea (see [9] Section 6.6 p. 280) is to deform the contour of integration in such a way that the modulus of the exponential integrand varies the most rapidly along it and then apply Laplace method to calculate the integral. It is shown in [9] (p. 287) that the paths of steepest ascent/descent coincide with paths where the imaginary part of the exponential factor of the integrand stays constant. Indeed, Cauchy-Riemann conditions imply orthogonality of real and imaginary parts and therefore isolines of the latter identify gradient directions of the former and thus of the modulus of the exponential.

In our case, the path in  $k$  extends from generic values of  $q$  (with  $|q| \gg 1$  as they are on the semicircles) in the complex plane to the first sextant. The exponential factor of the integrand is  $\rho(k) = ikx - sk - k^3/3$  and we analyze it in the neighborhood of the beginning  $k = q$  of the path. Since  $|q| \gg 1$ , the dominant contribution to  $\rho$  comes from the  $k^3$  term. Around  $k = q$ , we can expand  $k = |q|e^{i\theta} + |\delta k|e^{i\phi}$  (with  $|\delta k|$  small) and find

$$\text{Im}(k^3) \simeq |q|^3 \sin(3\theta) + 3|q|^2|\delta k| \sin(2\theta + \phi); \text{Re}(k^3) \simeq |q|^3 \cos(3\theta) + 3|q|^2|\delta k| \cos(2\theta + \phi). \quad (30)$$

The constancy of the imaginary part entails either  $\phi = -2\theta$  or  $\phi = \pi - 2\theta$ , which leaves us with the term at the exponential  $-\text{Re}(k^3)/3 \simeq -\text{Re}(q^3)/3 \mp |q|^2|\delta k|$ . For the convergence of the integral, the minus sign is needed and therefore the first option is the only possibility. Along this line, it holds that

$$|k| \simeq |q| + |\delta k| \cos(3\theta). \quad (31)$$

Let us now consider the various sextants. Referring to Fig. 1b in Ref. [1], we name I the first sextant  $-\pi/6 \leq \theta \leq \pi/6$ , II the sextant  $\pi/6 \leq \theta \leq \pi/2$ , and so on with the following ones in counterclockwise order and width  $\pi/3$  each. The first sextant is special because it is the only one where the path starts from  $q$  and moves outward, toward infinity, and not inward, as for all the others. Looking at the difference  $|k| - |q|$  in Eq. (31), we see that it is indeed negative for sextants II, IV and VI, whilst it is positive for sextants I, III, V. All the former ones admit then a path of steepest descent. As for the latter group, the only admissible sextant is I, as the path should point outward, whilst III and V do not admit a steepest descent path. For the admissible sextants, the integral to be calculated is  $\int_0^\infty e^{-|q|^2|\delta k|} d|\delta k|$ , where, as usual in asymptotic expansions, we have extended the integral to infinity as  $|q| \gg 1$ . The final result in the admissible sextants is  $\int_q^\infty e^{ikx} e^{-sk - k^3/3} dk \simeq e^{iqx} e^{-sq - q^3/3} / |q|^2$ , which yields the final expression (2.15) of Ref. [1].

As for our Eq. (22), the derivation goes through exactly in the same way. Indeed, since the whole analysis is based on the dominant  $k^3$  term, the  $r'$  terms is irrelevant, leaving Eq. (2.15) in Ref. [1] unaltered.

*a. Rotated contours and Airy functions.* It follows from Eq. (2.15) of Ref. [1] that we should use the upper circle  $C_1$  if  $x > y$  and the lower circle if  $x < y$ . Along the upper circle, the only non-vanishing contribution comes from the third sextant  $C_2 = (\pi/2, 5\pi/6)$ . Along the lower circle, it is the fifth sextant  $C_{-2} = (-5/6\pi, -\pi/2)$  which contributes. Let us express those contributions in terms of Airy functions. We remind that the Airy function  $Ai$  is defined as

$$Ai(x) = \frac{1}{2\pi i} \int_{C_{-5}-C_5} e^{xz - z^3/3} dz, \quad (32)$$

where the paths  $C_{-5}$  and  $C_5$  are defined in Fig. 1a of Ref. [1] and their subtraction  $C = C_5 - C_{-5}$  is a path starting at  $\infty e^{4/3i\pi}$  and finishing at  $\infty e^{2/3i\pi}$ . We define  $j \equiv e^{2/3i\pi}$ ; note that  $1/j = e^{-2/3i\pi} = j^2$ . By shifting  $z \mapsto z/j$  the path  $C$  is converted into  $C_5$  and by  $z \mapsto zj$  the path  $C$  goes into  $-C_{-5}$ . Since  $z^3 \mapsto z^3$  in both cases, we have

$$\frac{1}{2\pi i} \int_{C_5} e^{xz - z^3/3} dz = \frac{Ai(x/j)}{j}; \quad \frac{1}{2\pi i} \int_{-C_{-5}} e^{xz - z^3/3} dz = -j Ai(xj). \quad (33)$$

Note that in both cases contributions of the integrand at large values of  $q$  in the third and fifth sextant are negligibly small. It follows that cutting the integral at large values of  $q$  in the sextants is an exponentially small correction to the above values of the integral.

*b. Final formulæ for the resolvent.* With the help of the above formulae, the steps (2.20)-(2.23)b in Ref. [1] are straightforward. The modification for our Eq. (22) amounts to shifting  $s \mapsto s - r'$ , so that (2.23)a and (2.23)b become:

$$\begin{aligned} \hat{G}(x, y; s) &= 2\pi Ai\left(\frac{ix + r' - s}{j}\right) Ai(j(iy + r' - s)) \quad \text{for } x > y; \\ \hat{G}(x, y; s) &= 2\pi Ai\left(\frac{iy + r' - s}{j}\right) Ai(j(ix + r' - s)) \quad \text{for } x < y. \end{aligned} \quad (34)$$

The steps (2.24)-(2.26) in Ref. [1] are simple algebra on the expression (28). We can repeat the same steps on Eq. (29) for  $r' \neq 0$  to find what follows. We define

$$q \equiv \frac{u - t}{2}; \quad k = \frac{u + t}{2}. \quad (35)$$

Inserting into Eq. (29), we find

$$\hat{G}(x, y; s) = \frac{1}{4\pi} \int_{-\infty}^{+\infty} e^{iu/2(x-y) - u^2 t/4} du \int_0^\infty e^{-st} e^{r' t + it/2(x+y) - t^3/12} dt. \quad (36)$$

Completing the square and performing the resulting Gaussian integral over  $u$ , we obtain

$$\hat{G}(x, y; s) = \int_0^\infty \frac{1}{\sqrt{4\pi t}} e^{-st} e^{r't + it/2(x+y) - t^3/12 - \frac{(x-y)^2}{4t}} dt, \quad (37)$$

which yields for the Green's function  $G(x, y; t)$ :

$$G(x, y; t) = \frac{1}{\sqrt{4\pi t}} e^{r't + it/2(x+y) - t^3/12 - \frac{(x-y)^2}{4t}}. \quad (38)$$

The steps (2.27)-(2.31) in Ref. [1] are a rewriting of the expression (28) and the last step uses that the Laplace transform of  $\delta(t)$  is unity. The Heaviside constraint is automatically taken into account as  $\delta(k - q - t)$  enforces it since  $t \geq 0$ . For our case  $r' \neq 0$ , we get the following.

The Fourier transform of the resolvent is defined as

$$\hat{P}(k, q; s) = \frac{1}{2\pi} \int_{-\infty}^{+\infty} e^{-ikx + iqu} \hat{G}(x, y; s) dx dy, \quad (39)$$

and its inverse is

$$\hat{G}(x, y; s) = \frac{1}{2\pi} \int_{-\infty}^{+\infty} e^{ikx - iqu} \hat{P}(k, q; s) dk dq. \quad (40)$$

Inspection of Eq. (29) gives

$$\hat{P}(k, q; s) = \Theta(k - q) e^{-(k^3 - q^3)/3 - (s - r')(k - q)}, \quad (41)$$

where  $\Theta(\bullet)$  is the Heaviside step function. Taking the inverse Laplace transform, we obtain

$$P(k, q; t) = e^{-(k^3 - q^3)/3 + r'(k - q)} \delta(k - q - t). \quad (42)$$

Reestablishing the original dependencies on diffusivity  $D$ , frequency gradient  $g$  (which is taken positive here), and the original value of the growth rate  $r$  (the dimensional units of time and space are  $g^{-2/3}D^{-1/3}$  and  $(D/g)^{1/3}$ ), we obtain for the Green's function

$$G(x, y; t) = \frac{1}{\sqrt{4\pi Dt}} e^{rt + \frac{igt(x+y)}{2} - \frac{g^2 Dt^3}{12} - \frac{(x-y)^2}{4Dt}}. \quad (43)$$

The resolvent reads

$$\hat{G}(x, y; s) = \frac{1}{2\pi g} \int_{-\infty}^{+\infty} e^{-iqu} e^{\frac{(s-r)}{g}q + \frac{Dq^3}{3g}} dq \int_q^\infty e^{ikx} e^{-\frac{(s-r)}{g}k - \frac{Dk^3}{3g}} dk, \quad (44)$$

The spatial Fourier transform of the resolvent is

$$\hat{P}(k, q; s) = \frac{1}{g} \Theta(k - q) e^{-\frac{D}{3g}(k^3 - q^3) - \frac{(s-r)}{g}(k - q)}, \quad (45)$$

Finally, the momentum Green's function reads

$$P(k, q; t) = e^{-\frac{D}{3g}(k^3 - q^3) + \frac{r}{g}(k - q)} \delta(k - q - gt) = \delta(k - q - gt) e^{t(r - Dq^2) - Dqgt^2 - \frac{Dg^2 t^3}{3}}. \quad (46)$$

## 2. Asymptotic expansions of the Airy function $Ai$ for large arguments

The formulæ (3.5) and (3.6) of Ref. [1] involve the asymptotic expansion of the Airy function  $Ai$  for large arguments in the complex plane. The result that is needed is

$$Ai(x) \simeq \frac{1}{2\sqrt{\pi}} x^{-1/4} e^{-\frac{2}{3}x^{3/2}} \left[ 1 - \frac{5}{48x^{3/2}} + \dots \right] \quad \text{for } |\text{Arg}(x)| < \pi. \quad (47)$$

It follows then that

$$Ai(x) \rightarrow 0 \quad \text{for } 0 \leq |\text{Arg}(x)| < \frac{\pi}{3}; \quad Ai(x) \rightarrow \infty \quad \text{for } \frac{\pi}{3} < |\text{Arg}(x)| < \pi, \quad (48)$$

and (3.5) and (3.6) are finally obtained by using  $\text{Arg}(ie^{2i\pi/3}) = 7\pi/6$  and  $\text{Arg}(ie^{-2i\pi/3}) = -\pi/6$ .

Let us remind how Eq. (47) is obtained by the method of steepest descent [9]. The factor at the exponential of the definition Eq. (32) is  $\rho(z) = xz - z^3/3$ , which has a saddle point at  $z_*^2 = x$ . We take the argument  $\theta$  of  $x$  in the range  $-\pi < \theta < \pi$  so that  $z_* = |x|^{1/2}e^{i(\theta/2+\pi)}$  is the saddle point in the left half-plane. The value of the factor  $\rho(z_*) = -2x^{3/2}/3$  and its second derivative  $\rho''(z_*) = -2z_* = 2\sqrt{x}$ . The path of steepest descent is along the direction of constant imaginary part [9]. If we denote  $z - z_* = \delta z = |\delta z|e^{i\psi}$  then the imaginary part of  $\rho''(z_*)\delta z^2/2 = \sqrt{x}\delta z^2$  vanishes for  $2\psi + \theta/2 = 0$  or  $2\psi + \theta/2 = \pi$ . The former is a steepest ascent and the latter is steepest descent, which is what we need. The resulting integral is

$$Ai(x) \simeq \frac{1}{2\pi i} e^{-\frac{2}{3}x^{3/2}} \int_{-\infty}^{\infty} e^{-|x|^{1/2}|\delta z|^2} d|\delta z| e^{i\psi} e^{-\delta z^3/3}. \quad (49)$$

Since the Gaussian factor decreases rapidly, the last exponential can be expanded as  $\exp(-\delta z^3/3) \simeq 1 - \delta z^3/3 + \delta z^6/18 + \dots$ . The first unit term gives a Gaussian integral equal to  $e^{i\psi}\sqrt{\pi}/|x|^{1/2}$ , the second term vanishes by symmetry and the third yields the correction  $\frac{15}{18} \frac{e^{6i\psi}}{(2|x|^{1/2})^3} \frac{\sqrt{\pi}e^{i\psi}}{|x|^{1/4}}$ . Combining all the terms and recognizing that the value of the phase  $\psi = \pi/2 - \theta/4$  cancels the  $i$  at the denominator, reconstitutes the values of  $x$  and brings a minus sign for the correction, we obtain the expression (47).

## B. One reflecting boundary

The resolvent solves Eq. (24), which, for  $x \neq y$ , is the Airy equation with  $w = ix - s$ . We consider a domain extending on the right to infinity and having one reflecting boundary at  $x = \ell$ . In view of the structure of the resolvent Eq. (34), it is convenient to look for a solution in the form

$$\hat{G}(x, y; s) = \begin{cases} A Ai(w/j) + B Ai(jw) & \text{for } x < y, \\ C Ai(w/j) + D Ai(jw) & \text{for } x > y. \end{cases} \quad (50)$$

The coefficient  $D$  must vanish for the condition at infinity (see the asymptotic behaviors above). At  $x = y$  the two expressions should be continuous and have a jump in the derivative equal to  $-1$  (see Eq. (24)). At  $x = \ell$ , the derivative should vanish. Equations (3.9)-(3.13) of Ref. [1] follow.

Solving the three equations for the three unknowns  $A$ ,  $B$  and  $C$ , we obtain:

$$A = -2\pi j^2 Ai\left(\frac{w_y}{j}\right) \frac{Ai'(jw_\ell)}{Ai'\left(\frac{w_\ell}{j}\right)}; \quad B = 2\pi Ai\left(\frac{w_y}{j}\right); \quad C = 2\pi \left[ Ai(w_y j) - j^2 \frac{Ai\left(\frac{w_y}{j}\right) Ai'(jw_\ell)}{Ai'\left(\frac{w_\ell}{j}\right)} \right]. \quad (51)$$

To simplify the expression of  $A$ , we have used the Wronskian, which is derived hereafter, and the property  $j^3 = 1$ , which entails  $1/j = j^2$ . Plugging the expressions of the coefficients into Eq. (50) and subtracting the open-boundary expression (34), we obtain (3.15) of Ref. [1]. The difference (3.15) vanishes as  $\ell \rightarrow -\infty$  since  $Ai'\left(\frac{w_\ell}{j}\right) \rightarrow \infty$  (see the above asymptotic expansions), which is Eq. (3.16) of Ref. [1].

### 1. The Wronskian

The Wronskian (3.17) is obtained as follows. From the Airy equation, it follows that the Wronskian of two solutions  $f_1$  and  $f_2$  of the Airy equation

$$W(f_1, f_2) = f_1 f_2' - f_1' f_2, \quad (52)$$

satisfies the equation  $W' = 0$ , which is obtained by simple differentiation and using  $f_{1,2}'' = x f_{1,2}$ . If the two solutions are dependent, then the constant vanishes. In the case of  $f_1 = Ai(z/j)$  and  $f_2 = Ai(jz)$ , the solutions are independent

and the Wronskian reads  $j Ai(z/j) Ai'(jz) - Ai(jz) Ai'(z/j)/j = \text{const.} \equiv K$ . The constant is calculated taking, for instance, the values at the origin, where it is known that  $Ai(0) = \frac{1}{3^{2/3}\Gamma(2/3)}$  and  $Ai'(0) = -\frac{1}{3^{1/3}\Gamma(1/3)}$ . It follows that the constant

$$K = \frac{1}{3\Gamma(2/3)\Gamma(1/3)} \left( \frac{1}{j} - j \right) = \frac{\sin(\pi/3)}{3\pi} 2i \sin(-2/3\pi) = -\frac{i}{2\pi} = -\frac{j^{3/4}}{2\pi}. \quad (53)$$

For the second equality, we have used the identity  $\Gamma(x)\Gamma(1-x) = \frac{\pi}{\sin(\pi x)}$  and the last step is used in Ref. [1] to obtain an expression that is invariant under the exchange  $j \mapsto 1/j$ , which reverses the order in the Wronskian (and therefore the sign) and  $j^{3/4}$  changes sign as well.

## 2. Poles of the resolvent and stability

Poles of the resolvent are located at those values where the denominator  $Ai' \left( \frac{w_\ell}{j} \right)$  vanishes, that is  $i\ell - s = ja'_n$  where  $a'_n$  are the zeros of the derivative  $Ai'$ . Its zeros (as well as those of  $Ai$ ) are on the negative real axis (see [15] page 15 or [16] page 450). We therefore have singularities at  $s = i\ell - ja'_n$ , the real part of which is  $-a'_n \cos(2/3\pi) = a'_n/2 < 0$ . The system is therefore stable (remember the path of the inverse Laplace transform must run to the right of all singularities, so if they are all negative we can run it with a negative real part).

The residue of the resolvent at the pole (formulæ(3.20)-(3.21) in Ref. [1]) is:

$$Res = -2\pi e^{2i\alpha} Ai(e^{-i\alpha}(ix - s_{n_\alpha})) Ai(e^{-i\alpha}(iy - s_{n_\alpha})) Ai'(e^{i\alpha}(il - s_{n_\alpha})) \lim_{s \rightarrow s_{n_\alpha}} \frac{s - s_{n_\alpha}}{Ai'(e^{-i\alpha}(il - s))}, \quad (54)$$

where  $\alpha \equiv 2\pi/3$  in this Section to conform with Ref. [1]. The first derivative at the denominator can be expanded as

$$Ai'(e^{-i\alpha}(il - s)) \simeq 0 - Ai''(e^{-i\alpha}(il - s_{n_\alpha})) e^{-i\alpha}(s - s_{n_\alpha}) = -(s - s_{n_\alpha}) e^{-i\alpha} Ai(a'_n) a'_n. \quad (55)$$

Here, we have used the Airy equation  $Ai''(z) = z Ai(z)$ . One remark is worth. The function  $Ai(z)$  solves  $Ai''(z) = z Ai(z)$ . Since  $e^{3i\alpha} = 1$ , the two functions  $Ai(e^{\pm i\alpha} z)$  solve both  $d^2 Ai(z e^{\pm i\alpha})/dz^2 = z Ai(z e^{\pm i\alpha})$  (which is (3.3)) and  $d^2 Ai(z')/dz'^2 = z' Ai(z')$  where  $z' = e^{\pm i\alpha} z$ , which is what we used here. We can further simplify the expression of the residue by using the Wronskian (3.17) in Ref. [1] specified to the case  $z = i\ell - s_{n_\alpha}$ . The first term on the r.h.s. then vanishes and we obtain

$$\frac{e^{3i\alpha/4}}{2\pi} = -e^{i\alpha} Ai'(e^{i\alpha} z) Ai(e^{-i\alpha} z) \rightarrow Ai'(e^{i\alpha} z) = -\frac{e^{-i\alpha/4}}{2\pi Ai(e^{-i\alpha} z)} = -\frac{e^{-i\alpha/4}}{2\pi Ai(a'_n)}. \quad (56)$$

Combining the previous formulæ, we finally obtain (3.20)-(3.21) in Ref. [1]:

$$Res = -e^{11i\alpha/4} \frac{Ai(e^{-i\alpha}(ix - s_{n_\alpha})) Ai(e^{-i\alpha}(iy - s_{n_\alpha}))}{a'_n (Ai(a'_n))^2} = e^{-7i\alpha/4} \frac{Ai(e^{-i\alpha}(ix - s_{n_\alpha})) Ai(e^{-i\alpha}(iy - s_{n_\alpha}))}{a'_n (Ai(a'_n))^2}. \quad (57)$$

Equation (3.22) in Ref. [1] is the original Airy function (3.3) and the value of  $s = s_{n_\alpha}$  was identified as such that the no flux boundary condition at  $\ell$  was satisfied so (3.23) in Ref. [1] is obvious.

To obtain (3.24) in Ref. [1], one has to take the two Eqs. (3.23) for  $s = s_{n_\alpha}$  and  $s = s_{m_\alpha}$ , multiply the first by  $Ai(e^{-i\alpha}(ix - s_{m_\alpha}))$  and the second by  $Ai(e^{-i\alpha}(ix - s_{n_\alpha}))$ , integrate by parts, use the no flux boundary conditions  $Ai'(e^{-i\alpha}(ix - s_{m_\alpha, n_\alpha})) = 0$ , which leads to

$$(s_{n_\alpha} - s_{m_\alpha}) \int_\ell^\infty Ai(e^{-i\alpha}(ix - s_{m_\alpha})) Ai(e^{-i\alpha}(ix - s_{n_\alpha})) dx = 0, \quad (58)$$

that is the property of orthogonality between different pairs of functions. As for the normalization for  $m = n$ , the calculation goes as follows. By deriving the square  $Ai^2(z)$  and using that  $Ai'' = z Ai$  when the second derivative is encountered, we obtain that  $Ai''' = 4z(Ai(z)^2)' + 2Ai^2(z)$ , which is Eq. (10.4.57) of [16]. Integrating this equation from a point  $z_*$  where  $Ai'(z_*) = 0$  to infinity along a direction where  $Ai$  vanishes asymptotically, we obtain  $\int_{z_*}^\infty Ai^2(z) dz = -z_* Ai^2(z_*)$ . In our case  $z = e^{-i\alpha}(ix - s_{n_\alpha})$ , so that  $\int_\ell^\infty Ai^2(z) dx = \int_{a'_n}^{\infty e^{-i\pi/6}} Ai^2(z) dz e^{i\alpha - i\pi/2}$ . Note that the direction at infinity is within the angular sector of vanishing of  $Ai$  (see Eq. (48)). We conclude that

$$\int_\ell^\infty Ai^2(e^{-i\alpha}(ix - s_{n_\alpha})) dx = -a'_n Ai^2(a'_n) e^{i\alpha - i\pi/2} = a'_n Ai^2(a'_n) e^{7i\alpha/4}, \quad (59)$$

which is (3.24) of Ref. [1].

Eq. (3.25) in Ref. [1] is just the Laplace inverse transform, which picks all the poles. The sum is just given by the residues and the exponentials of the Laplace transform calculated at the poles.

If we add  $r'$  as in our Eq. (22), we get that the real part of  $s$  at the poles is  $r' + a'_n/2$ , which can become positive, i.e., the system can become linearly unstable. Reestablishing dimensional units, it should be the case that  $s = r + a'_n g^{2/3} D^{1/3}/2$  and the instability should kick in when

$$r > -a'_1 g^{2/3} D^{1/3}/2 \simeq 0.5094 g^{2/3} D^{1/3}. \quad (60)$$

A second unstable mode should kick in for  $r > -a'_2 g^{2/3} D^{1/3}/2 \simeq 1.6241 g^{2/3} D^{1/3}$ .

To directly compare with the dash-dotted line in Fig. 3 of the main text, we remind the definition of the non-dimensional parameter  $\beta \equiv \frac{Dg^2}{r^3}$  in Eq.(4) of the main text. It follows that Eq. (60) is equivalent to the condition

$$\beta < \left( \frac{1}{0.5094} \right)^3 \simeq 7.565, \quad (61)$$

for instability, which is the dash-dotted line in Fig. 3C. The prediction becomes appropriate and relevant when the size of the domain  $L$  is large, i.e., for the right-hand side of the phase space portrait in Fig. 3C where it is indeed confirmed by the data.

- 
- [1] S. D. Stoller, W. Happer, and F. J. Dyson, Transverse spin relaxation in inhomogeneous magnetic fields, *Phys. Rev. A* **44**, 7459 (1991).
  - [2] N. Diamant and A. Bortoff, Nature of the intestinal low-wave frequency gradient, *Am. J. of Physiology-Legacy Content* **216**, 301 (1969).
  - [3] A. Rohatgi, *WebPlotDigitizer* (2024), version 5.2. <https://automeris.io>.
  - [4] G. V. Osipov and M. M. Sushchik, The effect of natural frequency distribution on cluster synchronization in oscillator arrays, *IEEE Trans. Circ. Sys. I: Fund. Theor. Appl.* **44**, 1006 (1997).
  - [5] G. Osipov and M. Sushchik, Synchronized clusters and multistability in arrays of oscillators with different natural frequencies, *Phys. Rev. E* **58**, 7198 (1998).
  - [6] A. A. Akopov, T. E. Vadivasova, V. V. Astakhov, and D. D. Matyushkin, Partial synchronization in inhomogeneous autooscillatory media, *Tech. Phys. Lett.* **29**, 629 (2003).
  - [7] V. S. Anishchenko, A. A. Akopov, T. E. Vadivasova, and G. I. Strelkova, Mechanisms of chaos onset in an inhomogeneous medium under cluster synchronization destruction, *New J. Phys.* **8**, 84 (2006).
  - [8] M. Ankerst, M. M. Breunig, H.-P. Kriegel, and J. Sander, Optics: ordering points to identify the clustering structure, *SIGMOD Rec.* **28**, 49–60 (1999).
  - [9] C. M. Bender and S. A. Orszag, *Advanced mathematical methods for scientists and engineers* (Springer New York, New York, NY, 1999).
  - [10] G. B. Ermentrout and N. Kopell, Frequency plateaus in a chain of weakly coupled oscillators, i., *SIAM J. Math. Anal.* **15**, 215 (1984).
  - [11] N. Kopell and G. B. Ermentrout, Symmetry and phaselocking in chains of weakly coupled oscillators, *Commun. Pure Appl. Math.* **39**, 623 (1986).
  - [12] H. Daido, Complexity and scaling of frequency plateaus in chains of coupled nonlinear oscillators, *Progr. Theor. Phys* **102**, 197 (1999).
  - [13] F. Bloch, Nuclear induction, *Phys. Rev.* **70**, 460 (1946).
  - [14] H. C. Torrey, Bloch equations with diffusion terms, *Phys. Rev.* **104**, 563 (1956).
  - [15] O. Vallée and M. Soares, *Airy functions and applications to physics* (World Scientific, Hackensack, NJ, 2004).
  - [16] M. Abramowitz and I. A. Stegun, *Handbook of Mathematical Functions with Formulas, Graphs, and Mathematical Tables* (Dover, 1964).
